# Supplementary material for: Spin Dynamics in Hybrid Halide Perovskites -- Effect of Dynamical and Permanent Symmetry Breaking
Source: arXiv:2409.13200 source file (2024-09-20)
Supplement: Supplementary file 1 [file SI-Sep18.pdf]

# Supplementary Material for: Spin Dynamics in Hybrid Halide Perovskites - Effect of Dynamical and Permanent Symmetry Breaking

Kejun Li,[1,2] Junqing Xu,[3] Uyen N. Huynh,[4] Rikard Bodin,[4] Mayank Gupta,[2] Christian Multunas,[5] Jacopo Simoni,[2] Ravishankar Sundararaman,[6] Zeev Valy Verdany,[4] and Yuan Ping[2,7,8,*]

[1] *Department of Physics, University of California, Santa Cruz, California, 95064, United States*
[2] *Department of Materials Science and Engineering, University of Wisconsin-Madison, 53706, United States*
[3] *Department of Physics, Hefei University of Technology, Hefei, Anhui, China*
[4] *Department of Physics and Astronomy, University of Utah, Salt Lake City, UT, 84112, United States*
[5] *Department of Physics, Rensselaer Polytechnic Institute, 110 8th Street, Troy, New York 12180, United States*
[6] *Department of Materials Science and Engineering, Rensselaer Polytechnic Institute, 110 8th Street, Troy, New York 12180, United States*
[7] *Department of Physics, University of Wisconsin-Madison, Madison, Wisconsin 53706, United States*
[8] *Department of Chemistry, University of Wisconsin-Madison, Madison, Wisconsin 53706, United States*

(Dated: September 18, 2024)

## I. SPIN LIFETIME OF ELECTRONS IN $MAPbBr_3$ AT $B = 0$

Fig. S1 shows that electron-phonon scattering is dominant when temperature is higher than 10 K. Below 10 K, electron-impurity becomes significant to spin relaxation.

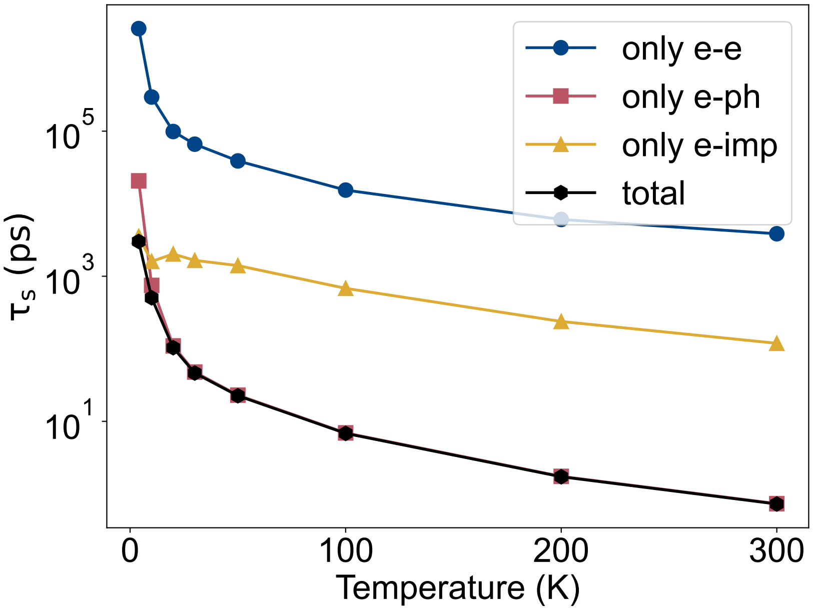


FIG. S1: Individual contributions of electron-electron (e-e), electron-phonon (e-ph) and electron-impurity (e-imp) scatterings to the spin lifetime, respectively. Both electron carrier density $n_e$ and impurity density $n_i$ are $10^{18}$ $cm^{-3}$. Pb vacancy defect $V_{Pb}$ is considered in the e-imp scattering in this work.

---

* yping3@wisc.edu

## II. ELECTRONIC STRUCTURE OF $MAPbBr_3$

Fig. S2 shows that Pb(s), Pb(p), Br(s) and Br(p) orbitals are major contributors to the band structure at the band edges. The MA molecules comprised of C, N and H atoms have negligible weight in the band structure at the band edges.

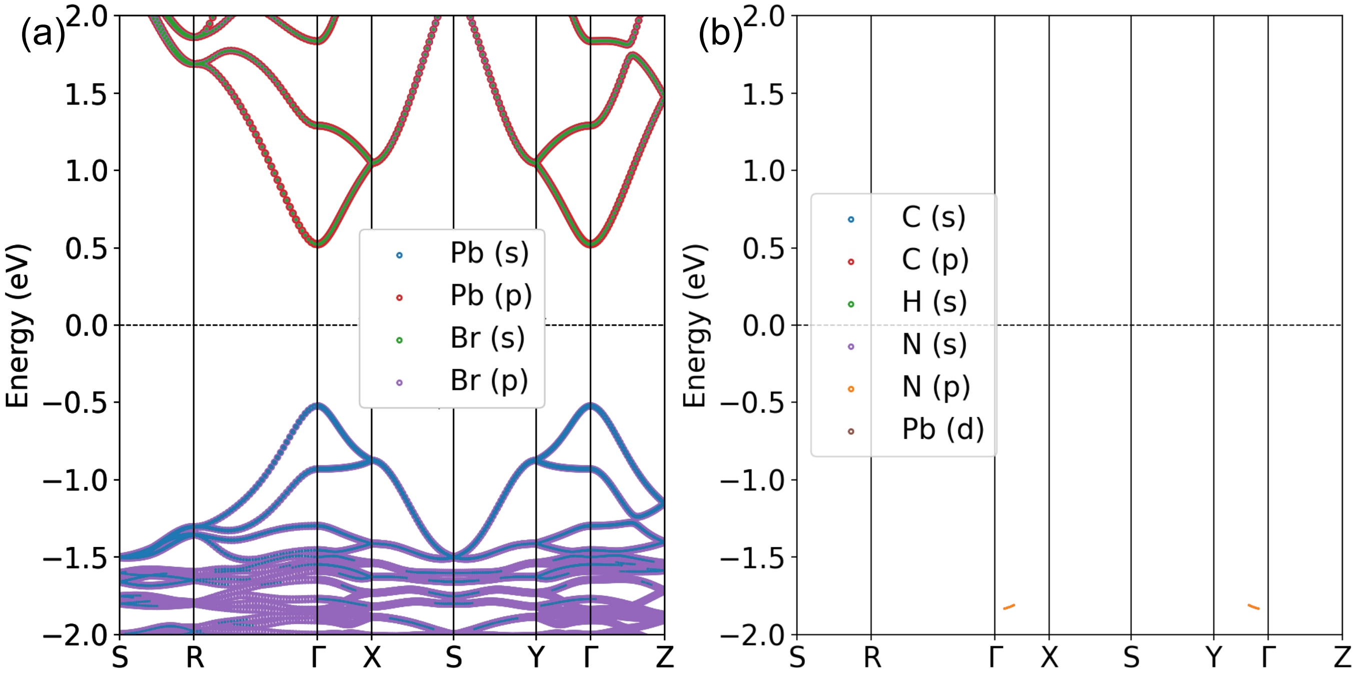


FIG. S2: (a) Orbital-projected band structure of $MAPbBr_3$ with respect to Pb(s), Pb(p), Br(s) and Br(p) orbitals. (b) Orbital-projected band structure of $MAPbBr_3$ with respect to C(s), C(p), H(s), N(s), N(p) and Pb(d) orbitals.

## III. SPIN RELAXATION MECHANISM OF THE SYMMETRIC $MAPbBr_3$

Without considering the hyperfine interaction, there are predominantly the Elliot-Yafet (EY) mechanism [1, 2] and Dyakonov-Perel (DP) mechanism contributing to the spin relaxation at the zero magnetic field. In particular, EY mechanism states that the spin relaxation time is proportional to the carrier lifetime. In contrast, the DP mechanism states that the spin relaxation time is inversely proportional to the carrier lifetime. Because the carrier relaxation rate scales linearly with the strength of electron scattering with electron, phonon or impurity, we can find the following relationship which is useful for identifying the mechanism for spin relaxation,

- EY mechanism ($\tau_s = \tau_p/4b^2$): ${\tau_s}^{-1} = {\tau_{s0}}^{-1} * A_{\text{scale}}$
- DP mechanism (${\tau_s}^{-1} \propto \tau_p \Delta\Omega^2$): ${\tau_s}^{-1} = {\tau_{s0}}^{-1}/A_{\text{scale}}$

where ${\tau_{s0}}^{-1}$ is the spin relaxation rate when the scattering matrix scaling factor $A_{\text{scale}}$ equals to 1. The scaling factor is defined in Eq. (1), and how it affects the time evolution of the electron density is in Eq. (2). By scaling the scattering, we find the line of the spin relaxation rate overlaps with that of EY mechanism. Therefore, we can determine the major mechanism to be the EY mechanism.

$$\widetilde{P}^c = A_{\text{scale}} P^c \tag{1}$$

$$\frac{d\rho_{12}}{dt} = \frac{1}{2}\sum_{345}\left[(I-\rho)_{13}\widetilde{P}^c_{32,45}\rho_{45} - (I-\rho)_{45}\widetilde{P}^{c,*}_{45,13}\rho_{32}\right] + H.C. \tag{2}$$

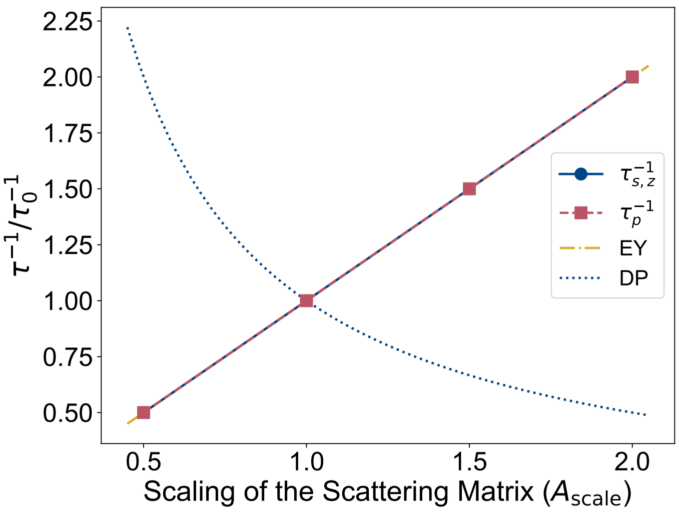


FIG. S3: The spin relaxation mechanism of the centrosymmetric $MAPbBr_3$ at 300 K under zero magnetic field and at the carrier density of $10^{18}$ $cm^{-3}$. The spin relaxation rate, carrier relaxation rate, and EY model scale linearly with the scaling factor $A_{scale}$ with slope=1. The DP mechanism scales inversely with the scaling factor $A_{scale}$.

## IV. PHONON AND ELECTRON-PHONON SCATTERING OF $MAPbBr_3$

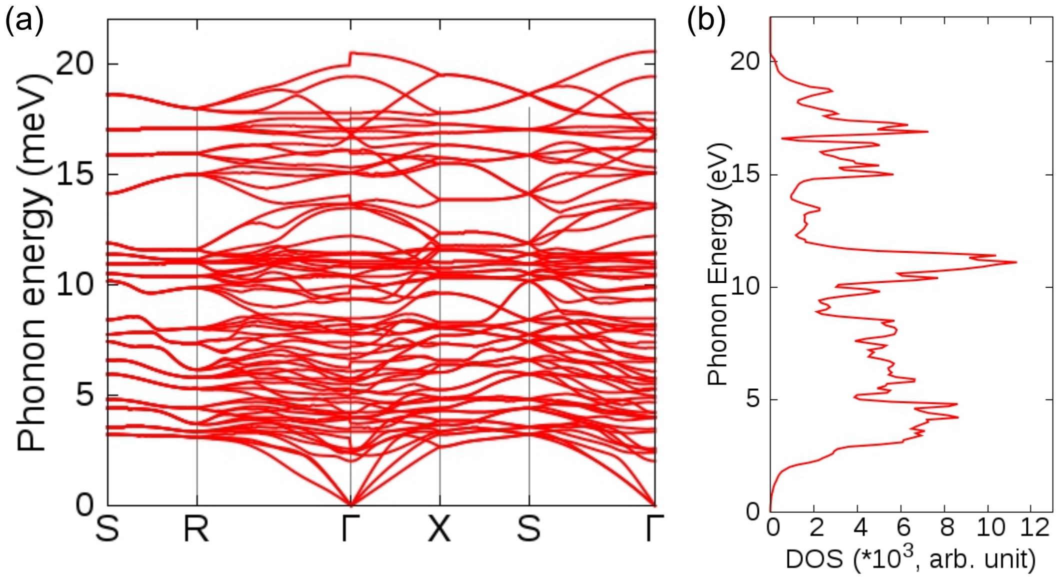


FIG. S4: (a) Phonon dispersion and (b) phonon density of states within the energy range of 24 meV of $MAPbBr_3$. The number of phonon modes is 72 within this energy range.

### A. Phonon Contribution

As electron-phonon scattering is the major scattering process in a wide range of temperatures, we focus on the contribution of electron-phonon (e-ph) coupling to carrier relaxation and spin relaxation (EY mechanism). These relaxation processes can be described by the simplified picture of Fermi's golden rule (FGR). $\tau_p^{-1}$ ($\tau_s^{-1}$) is proportional to the modulus square of the spin-conserving (spin-flip) electron-phonon scattering matrix element. The spin-conserving electron-phonon matrix element ($\overline{|\widetilde{g}^{\uparrow\uparrow}|^2}$) is analogue to the spin-flip one ($\overline{|\widetilde{g}^{\uparrow\downarrow}|^2}$) in terms of the form. Below, we

explicitkly write down the spin-flip e-ph matrix element,

$$\overline{|\widetilde{g}^{\uparrow\downarrow}|^2} = \frac{\sum_{kq} \mathrm{w}_{k,k-q} \sum_{\lambda} |g_{k,k-q}^{\uparrow\downarrow,q\lambda}|^2 n_{q\lambda}}{\sum_{kq} \mathrm{w}_{k,k-q}}, \tag{3}$$

$$\mathrm{w}_{k,k-q} = f_{k-q}\left(1-f_k\right)\delta\left(\epsilon_k - \epsilon_{k-q} - \omega_c\right), \tag{4}$$

where $g_{k,k-q}^{\uparrow\downarrow,q\lambda}$ is e-ph matrix element, accounting for an electron scattering from $\mathbf{k}$ to $\mathbf{k}-\mathbf{q}$, with phonon of mode $\lambda$ and wavevector $q$, with opposite spin. $n_{q\lambda}$ is phonon occupation. $f_k$ is Fermi-Dirac function. $\mathrm{w}_{k,k-q}$ is the weight function. $\omega_c$ is the characteristic phonon energy, which is set to, for example, 4 meV at 10 K based on our analysis of phonon-mode-resolved contribution to spin relaxation.

The $q$-dependent modulus square of the spin-flip e-ph matrix element $|\widetilde{g}^{\uparrow\downarrow}|^2\left(q\right)$ is written as

$$|\widetilde{g}^{\uparrow\downarrow}|^2\left(q\right) = N_k^{-1} \sum_{k\lambda} |g_{k,k-q}^{\uparrow\downarrow,q\lambda}|^2 n_{q\lambda}. \tag{5}$$

In particular, only states around the band edges are involved in spin relaxation. Thus we restrict $|\epsilon_k - \epsilon_{\mathrm{edge}}| <$180 meV for the calculation of Eq. 5, which is about $7k_BT$ at 300 K relative to the band edge energy ($\epsilon_{\mathrm{edge}}$). More details about the spin-conserving electron-phonon matrix element and spin-flip electron-phonon matrix element can be found in Ref. [3].

The phonon of $MAPbBr_3$ spans a wide range of energy from 0 to 400 meV. We focus on the phonon modes within the energy range 0-24 meV, corresponding to the temperature range of study (from zero up to 300K). This energy range includes in total 72 phonon modes, which involve the vibration of both the inorganic sublattice and the molecules [4]. Above this energy range, the phonon modes mostly correspond to internal vibration of MA molecules. Because carriers near band edges are mostly composed by states from the inorganic sublattice according to the band structure in Fig. S2, they can be nearly isolated from the internal vibration of MA molecules. Therefore, the phonon modes above should be less important to the electron-phonon coupling responsible for carrier relaxation and spin relaxation.

The spin relaxation is primarily caused by lower-energy optical phonons from phonon mode 8 to 23 in the energy range from 2-6 meV, contrary to the common assumption that LO phonons via the Fröhlich interaction are the major contributors to spin relaxation [5–7]. Fig. S5(a) shows that several low-energy optical phonons significantly reduce the spin lifetime compared to others. This is demonstrated by the spin-flip electron-phonon matrix element in Fig. S6(a), which shows the phonons other than O54-O72 to be the major contribution. The different phonon contribution to spin relaxation can be attributed to the short-range nature of spin-phonon interaction as spin indirectly interacts with phonon via SOC. The phonon contribution to electron-phonon interaction in $MAPbBr_3$ is similar to that in $CsPbBr_3$ [3], but it involves more complex molecular-inorganic lattice hybrid vibrational modes due to the inclusion of the organic MA molecule in place of the Cs atom.

For carrier relaxation, we identify the LO (longitudinal optical) modes that have strong contribution to the corresponding spin-conserving electron-phonon matrix elements, as shown in Fig. S5(b). At 4 K, the acoustic modes are the most active, with some low-energy optical modes, contributing to the electron-phonon scattering that induces carrier relaxation and spin relaxation. In this regime, the hyperfine interaction and electron-impurity interaction can be stronger than the electron-phonon interaction, which we didn't include here explicitly. When temperature increases (T > 10 K), more optical phonons of higher energy become thermally active. Especially when T > 50 K, the number 54 to 72 optical phonons become activated and have large contribution to carrier relaxation through spin-conserving electron-phonon scattering process, as shown by the spin-conserving matrix element in Fig. S6(b). Related to these optical phonon modes, as can be seen in Fig. S4(a), there occurs a large LO-TO splitting at $13-21$ meV, consistent with the strong Raman intensity at 12.3 meV, 12.6 meV, 16.2 meV and $22.3 \pm 0.6$ meV [8, 9]. They resulting in Fröhlich interaction via electron coupling with the LO phonons [10].

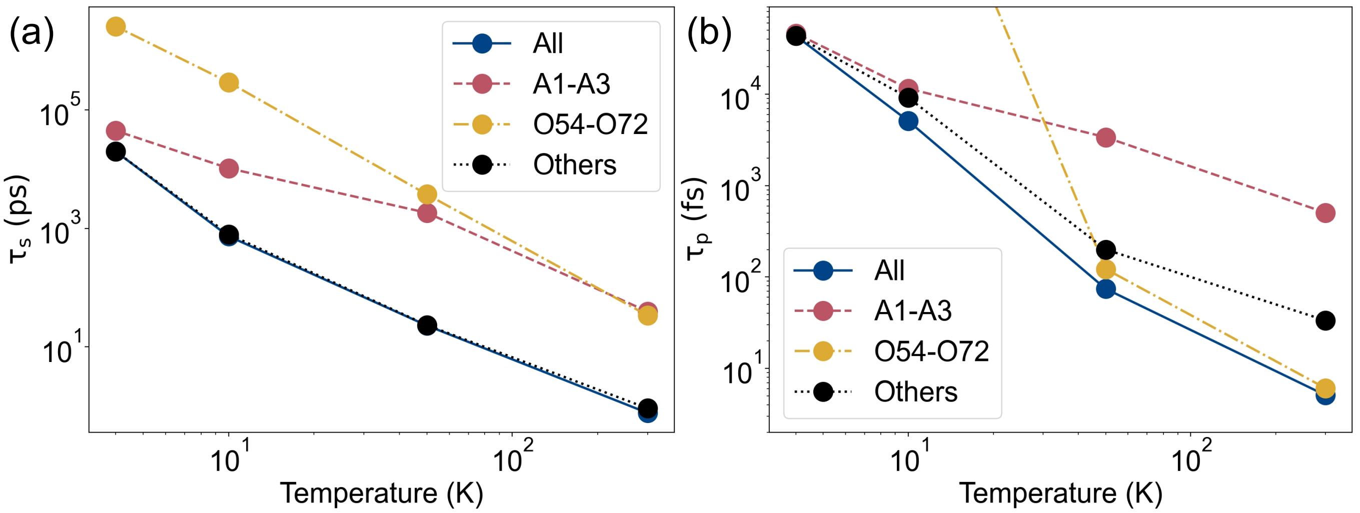


FIG. S5: (a) Temperature dependent spin relaxation time $\tau_s$ and (b) carrier relaxation time $\tau_p$. Phonon modes are separated into different groups in order to discern the major phonons that contribute to the electron-phonon interaction for $\tau_p$ and $\tau_s$. "All" represents the contribution from all phonons, A1-A3 represents three acoustic phonons, "O54-O72" represents the number 54 to 72 optical modes, and "Others" represents the other phonons aside from "A1-A3" and "O54-O72". The shorter the lifetime, the larger the phonon contribution.

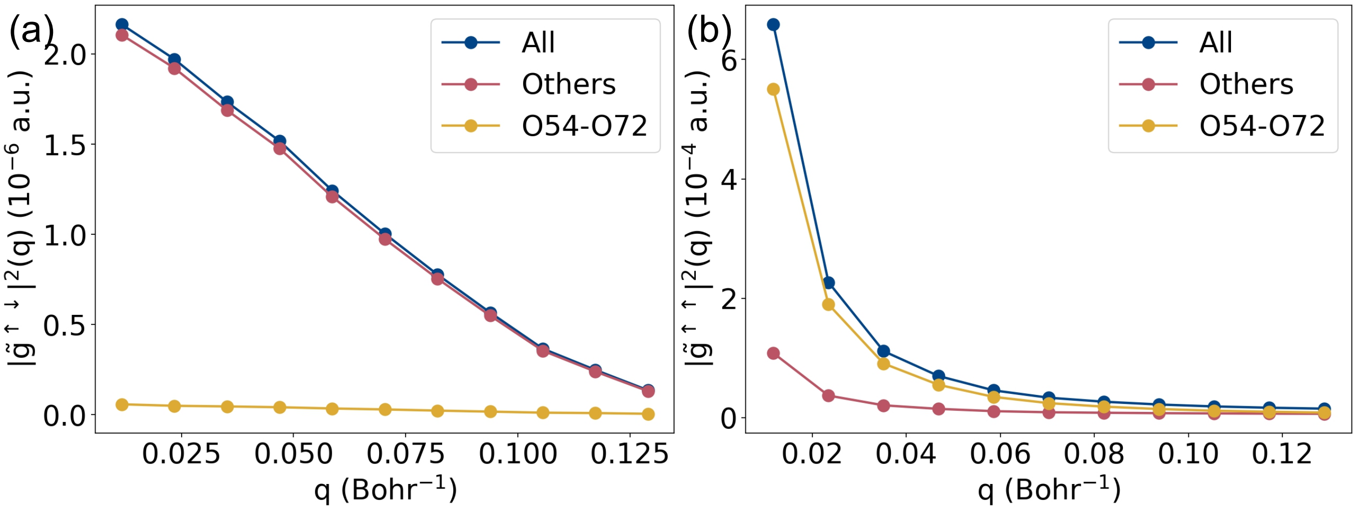


FIG. S6: (a) The q-dependent modulus square of the spin-flip electron-phonon matrix element $|g^{\uparrow\downarrow}|(q)$ for spin relaxation. (b) The q-dependent modulus square of the spin-conserving electron-phonon matrix element $|g^{\uparrow\uparrow}|(q)$ for carrier relaxation. Phonon modes are separated into different groups in order to discern the major phonons that contribute to the electron-phonon interaction for $\tau_p$ and $\tau_s$. "All" represents the contribution from all phonons, "O54-O72" represents the number 54 to 72 optical modes, and "Others" represents the other phonons aside from "O54-O72".

## V. $g$ FACTOR CALCULATION FROM FIRST-PRINCIPLES OF $MAPbBr_3$

The method for evaluating the $g$ factor from first-principles calculations is described in Ref. [3].

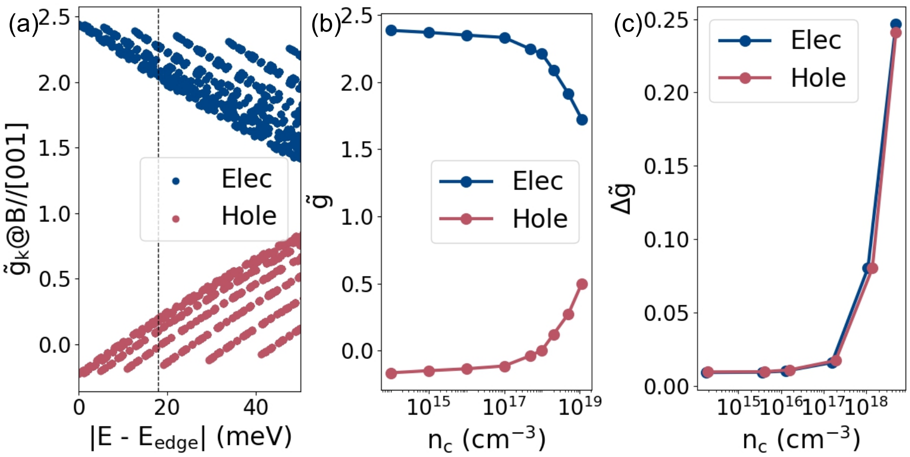


FIG. S7: (a) The k-dependent g factor $\tilde{g}_k$ evaluated with an external magnetic field along [001], as a function of energy or chemical potential near the band edge of $MAPbBr_3$. Each data point represents a g factor at a k point. The dashed line represent the Fermi level in the conduction band, at which the corresponding electron carrier density $n_c = 10^{18}$ cm$^{-3}$. (b) The statistically-averaged g factor as a function of carrier density at 4 K. (c) The fluctuation/variation of g factor as a function of carrier density at 4 K.

## VI. COEFFICIENTS FOR INTERNAL MAGNETIC FIELD

To analyze the internal magnetic field and spin texture, we adopt the following Hamiltonian, which describes the interaction between spin and internal magnetic field. The k space region considered is near the band edge minimum or maximum, where there is linear dependence of $\mathbf{B}^{\text{in}}$ and $\mathbf{k}$ when we expand around the band edge $\mathbf{k}$ point. In atomic unit,

$$H = \sigma^T \cdot C \cdot \mathbf{k} \tag{6}$$

where $\mathbf{k} = (k_x, k_y, k_z)$ as a column vector, $\sigma = (\sigma_x, \sigma_y, \sigma_z)$ as a column vector of Pauli's matrices for spin operators, and $C$, a coefficient tensor, is a $3 \times 3$ matrix.

By definition, the internal magnetic field is then $\mathbf{B}^{\text{in}} = C \cdot \mathbf{k}$ as a general linear function of $\mathbf{k}$. We can fit numerical data for $\mathbf{B}^{\text{in}}(\mathbf{k})$ to directly extract a $3 \times 3$ matrix $C$.

To analyze this matrix, let us consider the general transformation sectors within $C$. We can write any $3 \times 3$ matrix as:

$$C = \underbrace{C_s}_{\text{(scalar part)}} + \underbrace{C_v}_{\text{(anti-symmetric vector part)}} + \underbrace{C_t}_{\text{(traceless-symmetric tensor part)}} . \tag{7}$$

The first term is so-called Weyl contribution which is scalar.

$$C_s = \mathbb{1} * \text{Tr}(C)/3 \tag{8}$$

The second term is the antisymmetric Rashba contribution, $\mathbf{B}^{\text{in}}(\mathbf{k}) = (C_x, C_y, C_z) \times k$.

$$C_v = \begin{pmatrix} 0 & -C_z & C_y \\ C_z & 0 & -C_x \\ -C_y & C_x & 0 \end{pmatrix} \tag{9}$$

The third term is the symmetric Dresselhaus contribution (only take the linear order), which has five independent terms because $C_{xx} + C_{yy} + C_{zz} = 0$ (since trace taken out in $C_s$).

$$C_t = \begin{pmatrix} C_{xx} & C_{xy} & C_{xz} \\ C_{xy} & C_{yy} & C_{yz} \\ C_{zx} & C_{yz} & C_{zz} \end{pmatrix} \tag{10}$$

To simplify the picture by taking an example of two-dimensional SOC Hamiltonian, we have:

$$C_{t,2D} = \begin{pmatrix} C_{xx} & C_{xy} \\ C_{xy} & -C_{xx} \end{pmatrix} \tag{11}$$

Expanding out the Hamiltonian we would have:

$$H_{2D} = C_{xx}(\sigma_x k_x - \sigma_y k_y) + C_{xy}(\sigma_x k_y + \sigma_y k_x) \tag{12}$$

where the two terms are exactly the two different 2D Dresselhaus forms above.

To quantify the relative contribution of Rashba and Dresselhaus to the total coefficient tensor, a Dresselhaus/Rashba ratio $\mathcal{Q}$ is evaluated,

$$\mathcal{Q} = \frac{\sqrt{\sum_{ij} |C_{t;ij}|^2}}{\sqrt{\sum_{ij} |C_{v;ij}|^2}} \tag{13}$$

## VII. RASHBA SPLITTING COEFFICIENT FROM BAND SPLITTING IN BAND STRUCTURE OF $MAPbBr_3$

The Bychkov-Rashba Hamiltonian accounts for the Rashba effect originated from the inversion symmetry breaking, which can be expressed as [11]

$$H_{\text{Rashba}} = \frac{\mathbf{p}_{\|}^2}{2m} + \frac{\alpha' \hbar E_z}{4m_0^2 c^2}(\sigma \times \mathbf{p}_{\|}) \cdot \hat{z} \tag{14}$$

where $\mathbf{p}_{\|}$ is momentum in x-y plane, $m$ is relativistic mass, $m_0$ is the rest mass, $\hbar$ is the Planck's constant, $c$ is the speed of light, $\alpha'$ is the Rashba primary correlation factor, $E_z$ is the electric field in z axis due to inversion symmetry breaking, $\sigma$ is the Pauli's matrix, and $\hat{z}$ is the unit vector in z axis.

The eigenvalues of the Hamiltonian are found to be

$$\varepsilon_{\pm}(k) = \frac{\hbar^2}{2m}k^2 \pm \alpha k \tag{15}$$

$$\alpha = \frac{\varepsilon_+ - \varepsilon_-}{2\Delta k} \tag{16}$$

where $\alpha$ is the Rashba splitting coefficient. By evaluation as shown in Fig. S8, we obtain $\alpha = 1.35$ eV Å. We note that this theory assumes the spin split is solely from Rashba spin-orbit coupling, but in practice other types such as the Dresselhaus SOC also contributes to SOC.

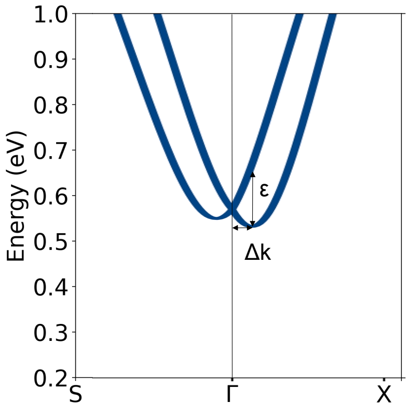


FIG. S8: The conduction band minimum of the asymmetric $MAPbBr_3$. $\varepsilon$ (0.13 eV) is the energy difference between the spitted bands at the vertex due to the Rashba effect, and $\Delta k$ (0.047 Å$^{-1}$) is the $k$ distance from the vertex to the reference high symmetry k point.

## VIII. BAND STRUCTURE OF $MPSnBr_3$

In Fig. S9, the spin polarized band structures indicate that the spin is mostly polarized in y-axis within a range (approximately 20% in Fig. S10) in the momentum space around high symmetry point X. This is found to be persistent spin helix (PSH).

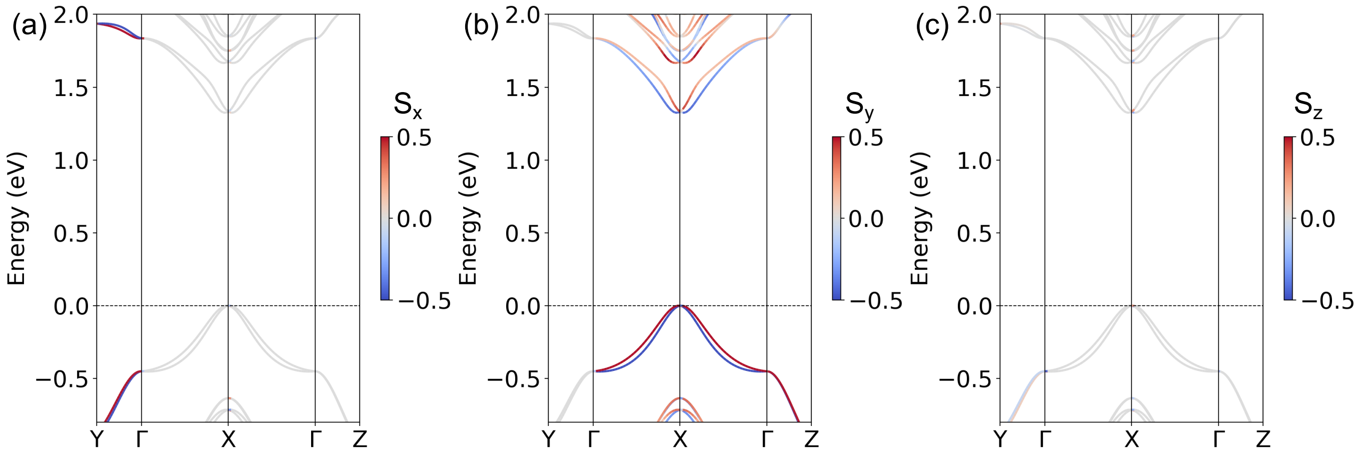


FIG. S9: Electronic band structures of $MPSnBr_3$ with spin polarization (a) $S_x$, (b) $S_y$, (c) $S_z$.

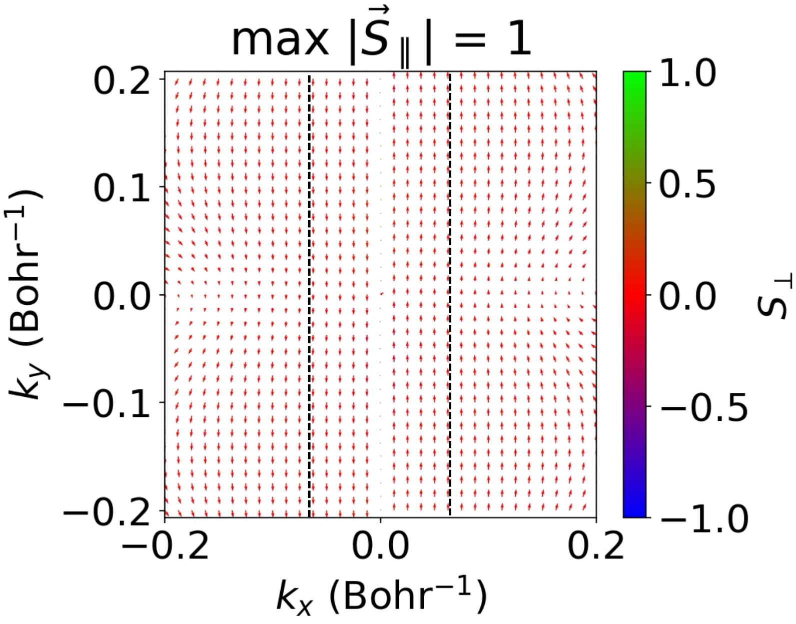


FIG. S10: Spin texture at the conduction band minimum (CBM) of $MPSnBr_3$. The region within the dashed lines visually indicates the presence of PSH. The width of the first Brillouin zone in x direction is 0.55 $\text{Bohr}^{-1}$.

## IX. PHONON DISPERSION OF $MPSnBr_3$

In the study of $MPSnBr_3$, we calculate the phonons by using the finite difference method implemented in JDFTx, with a k point mesh of $4 \times 2 \times 2$ and a q point mesh of $2 \times 2 \times 1$ . As shown in Fig. S4(a), the phonon energy is up to 385 meV due to the internal vibration of the MP molecules [12]. Zooming in the phonon dispersion within the energy range of 25 meV in Fig. S4(b), it can be found that there are small imaginary frequencies of the first two acoustic modes near Γ due to the instability of current structure. In current calculation of electron-phonon coupling for the

spin lifetime of $MPSnBr_3$, we include all phonon modes except the first two acoustic phonons, considering that at optical modes are the major contribution to the electron-phonon coupling at temperature higher than 50 K.

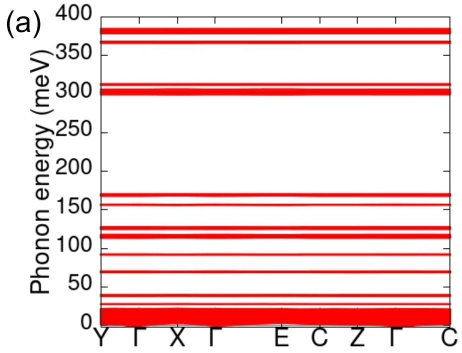


FIG. S11: Phonon dispersion of $MAPbBr_3$. (a) The full range of phonon dispersion calculated by using JDFTx. (b) Phonon dispersion within the energy range of 25 meV. The number of phonon modes is 70 within this range.

## X. PERSISTENT SPIN HELIX OF $MPSnBr_3$

We obtain the coefficient of the internal PSH magnetic field of $MPSnBr_3$ by using the method introduced in Sec. VI. The coefficient of determination is 0.98, confirming the validity of the linear relationship between $\mathbf{B}^{\text{in}}$ and $\mathbf{k}$. From the fitting of the internal magnetic field, we find that the Rashba and Dresselhaus contributions are nearly equal, with a Dresselhaus/Rashba ratio of 1.03 using Eq. (13), which is characteristic of PSH. Below are the specific coefficients in atomic units,

$$C_s = 5.09 \times 10^{-4} \tag{17}$$

$$C_v = \begin{pmatrix} 0 & -3.80 \times 10^{-2} & -1.95 \times 10^{-4} \\ 3.80 \times 10^{-2} & 0 & -1.07 \times 10^{-2} \\ 1.95 \times 10^{-4} & 1.07 \times 10^{-2} & 0 \end{pmatrix} \tag{18}$$

$$C_t = \begin{pmatrix} -3.20 \times 10^{-4} & 4.01 \times 10^{-2} & 9.90 \times 10^{-5} \\ 4.01 \times 10^{-2} & 6.52 \times 10^{-4} & -7.08 \times 10^{-3} \\ 9.90 \times 10^{-5} & -7.08 \times 10^{-3} & -3.32 \times 10^{-4} \end{pmatrix} \tag{19}$$

## XI. SPIN RELAXATION MECHANISM OF ELECTRONS IN $MPSnBr_3$

By the trend of spin relaxation rate with scaling the scattering matrix, we can find that the dominant mechanism of spin relaxation is EY mechanism, in particular in the y axis where there is PSH. In the direction perpendicular to the PSH, DP/FID mechanisms due to spin scattering or dephasing play a role.

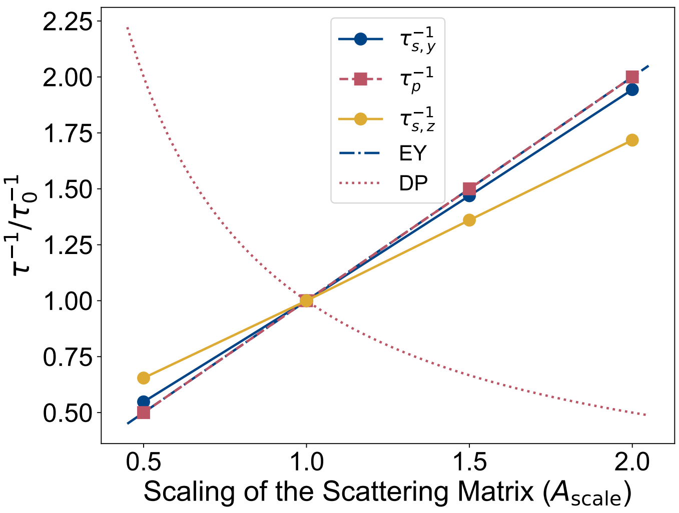


FIG. S12: The spin relaxation mechanism of electrons in $MPSnBr_3$ at 300 K under zero mangetic field and at the carrier density of $10^{18}$ $cm^{-3}$. The spin relaxation rate, carrier relaxation rate and EY mechanism scale linearly with the scaling factor $A_{scale}$. The DP mechanism scales inversely with the scaling factor $A_{scale}$.

## XII. SPIN LIFETIME OF HOLES IN $MPSnBr_3$

At the valence band maximum (VBM), the spin texture is Rashba-like. The spin lifetime of holes shows anisotropy similar to that of the asymmetric $MAPbBr_3$.

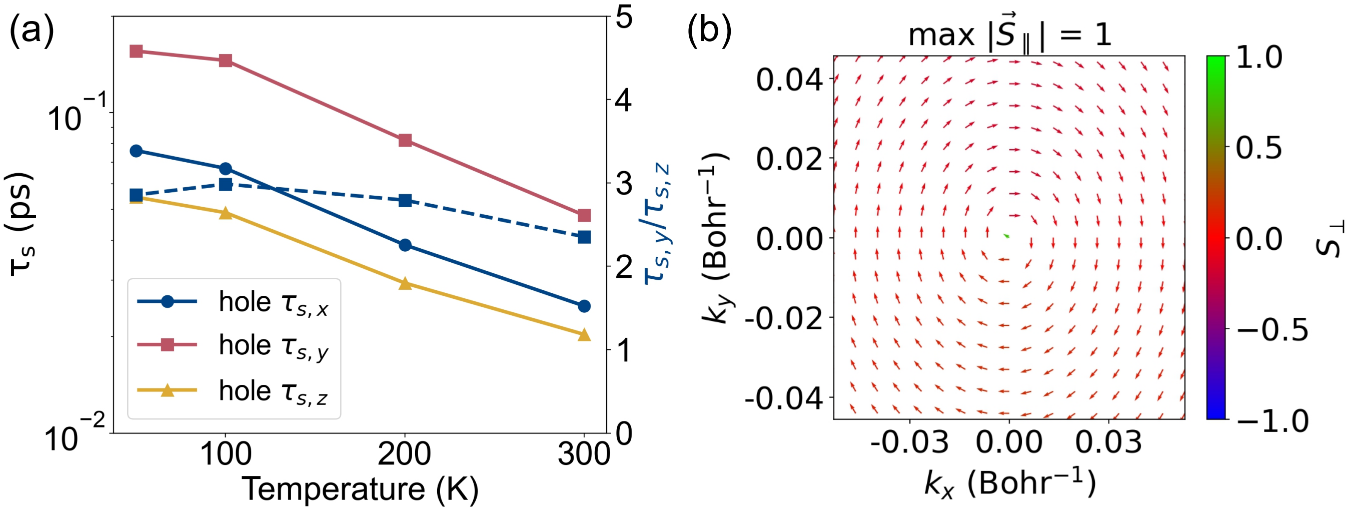


FIG. S13: (a) Temperature-dependent spin lifetime of holes in $MPSnBr_3$ at zero external magnetic field. (b) The Rashba spin texture at valence band maximum (VBM) centered at high symmetry point X. The red, blue and yellow data points with solid lines represent the spin lifetime of electrons in x, y and z direction. The data points with dashed lines are the anistropy of spin lifetime.


[1] I. Žutić, J. Fabian, and S. D. Sarma, Spintronics: Fundamentals and Applications, Rev. Mod. Phys. **76**, 323 (2004).
[2] J. Fabian and S. D. Sarma, Spin Relaxation of Conduction Electrons in Polyvalent Metals: Theory and a Realistic Calculation, Phys. Rev. Lett. **81**, 5624 (1998).

[3] J. Xu, K. Li, U. N. Huynh, M. Fadel, J. Huang, R. Sundararaman, V. Vardeny, and Y. Ping, How Spin Relaxes and Dephases in Bulk Halide Perovskites, Nat. Commun. **15**, 188 (2024).

[4] M. A. Pérez-Osorio, R. L. Milot, M. R. Filip, J. B. Patel, L. M. Herz, M. B. Johnston, and F. Giustino, Vibrational Properties of the Organic–Inorganic Halide Perovskite CH3NH3PbI3 from Theory and Experiment: Factor Group Analysis, First-Principles Calculations, and Low-Temperature Infrared Spectra, J. Phys. Chem. C **119**, 25703 (2015).

[5] V. V. Belykh, D. R. Yakovlev, M. M. Glazov, P. S. Grigoryev, M. Hussain, J. Rautert, D. N. Dirin, M. V. Kovalenko, and M. Bayer, Coherent Spin Dynamics of Electrons and Holes in CsPbBr3 Perovskite Crystals, Nat. Commun. **10**, 673 (2019).

[6] M. J. Crane, L. M. Jacoby, T. A. Cohen, Y. Huang, C. K. Luscombe, and D. R. Gamelin, Coherent Spin Precession and Lifetime-Limited Spin Dephasing in CsPbBr3 Perovskite Nanocrystals, Nano Lett. **20**, 8626 (2020).

[7] W. H. Sio and F. Giustino, Unified ab initio description of fröhlich electron-phonon interactions in two-dimensional and three-dimensional materials, Phys. Rev. B **105**, 115414 (2022).

[8] K. Matsuishi, T. Ishihara, S. Onari, Y. Chang, and C. Park, Optical Properties and Structural Phase Transitions of Lead-Halide Based Inorganic–Organic 3D and 2D Perovskite Semiconductors Under High Pressure, Phys. Stat. Sol. (b) **241**, 3328 (2004).

[9] M. Ledinský, P. Löper, B. Niesen, J. Holovský, S.-J. Moon, J.-H. Yum, S. De Wolf, A. Fejfar, and C. Ballif, Raman Spectroscopy of Organic–Inorganic Halide Perovskites, J. Phys. Chem. Lett. **6**, 401 (2015).

[10] M. Sendner, P. K. Nayak, D. A. Egger, S. Beck, C. Müller, B. Epding, W. Kowalsky, L. Kronik, H. J. Snaith, A. Pucci, *et al.*, Optical Phonons in Methylammonium Lead Halide Perovskites and Implications for Charge Transport, Mater. Horiz. **3**, 613 (2016).

[11] T. Etienne, E. Mosconi, and F. De Angelis, Dynamical origin of the rashba effect in organohalide lead perovskites: A key to suppressed carrier recombination in perovskite solar cells?, J. Phys. Chem. Lett. **7**, 1638 (2016).

[12] A. T. Eppink and D. Parker, Energy partitioning following photodissociation of methyl iodide in the a band: A velocity mapping study, J. Chem. Phys. **110**, 832 (1999).
